# Supplementary material for: Edit One for All: Interactive Batch Image Editing
Source: arXiv:2401.10219 source file (2024-01-18)

edit

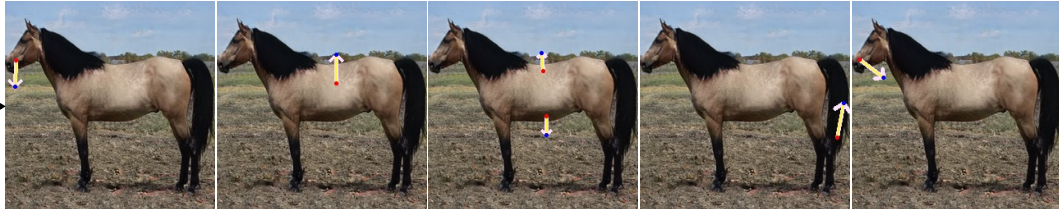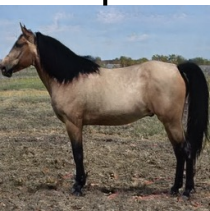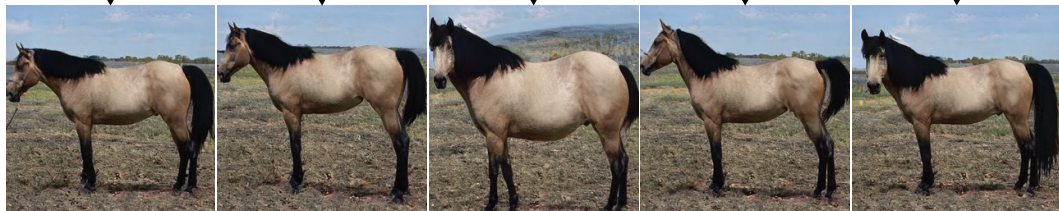

Example

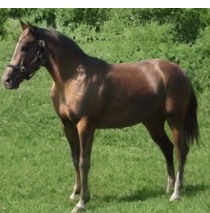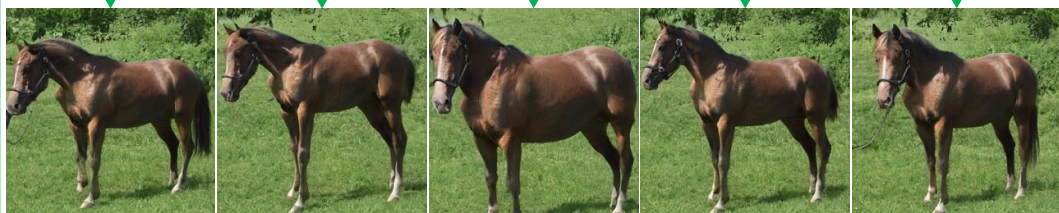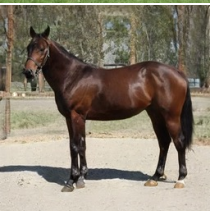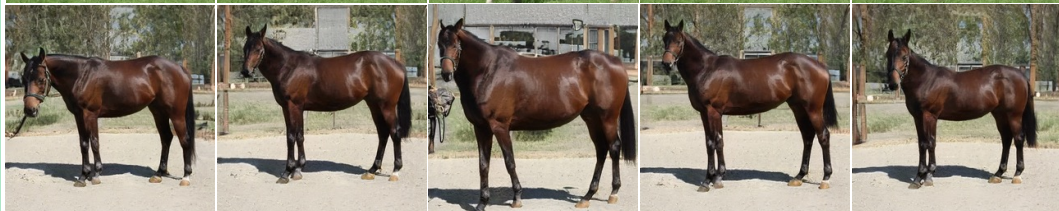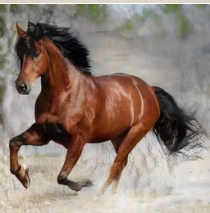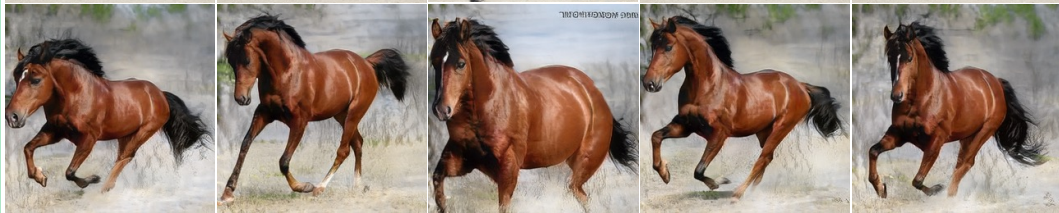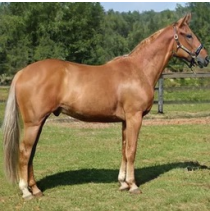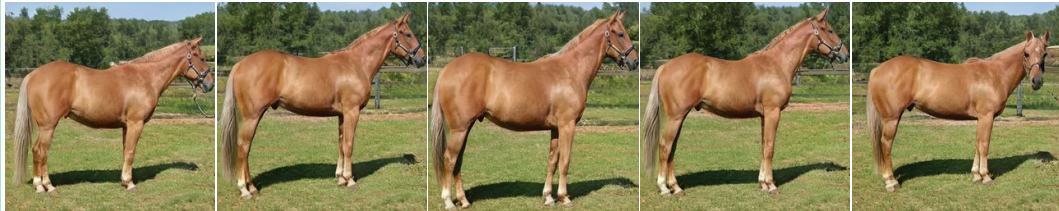

Test Images

Edited Images



edit

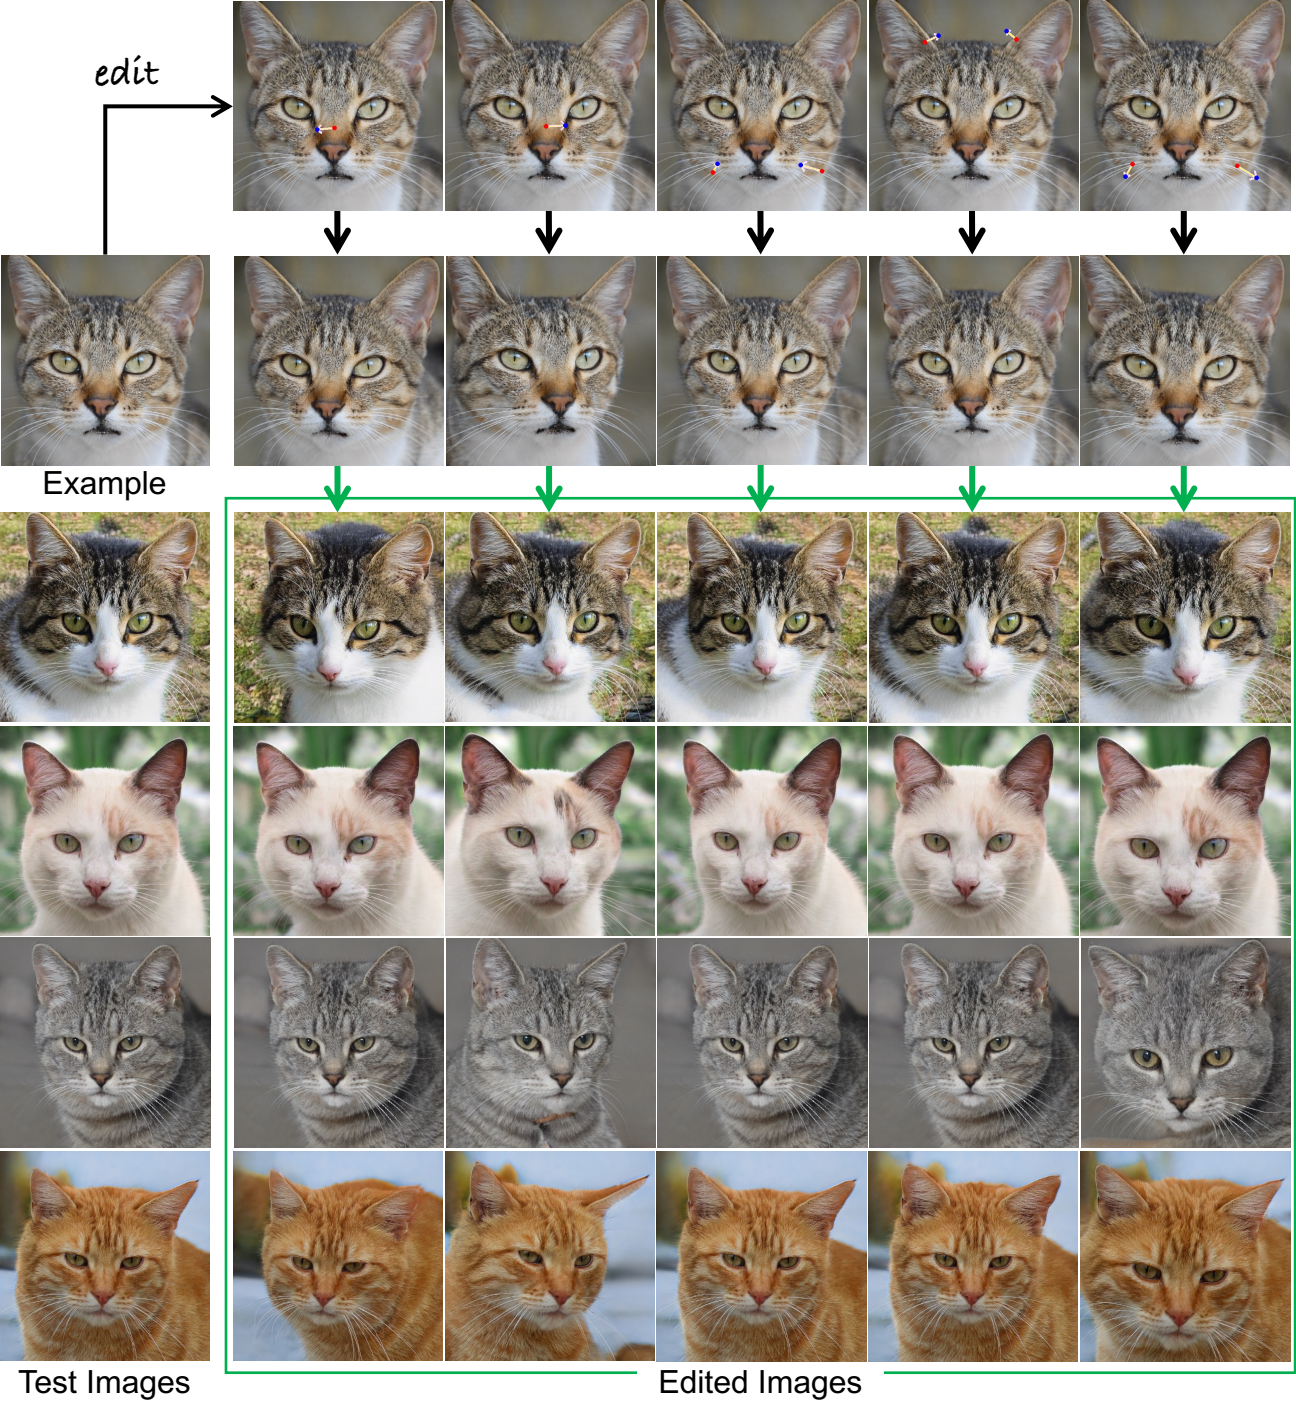

Supplement: Supplementary file 1 [file supp-extra-domain.pdf]
